# Supplementary material for: Framework and Tools for the Simulation and Analysis of the Radio Emission from Air Showers at IceCube
Source: arXiv:2205.02258 source file (2022-05-04)
Supplement: Supplementary file 1 [file Appendix1.tex]

\section{Efficiency Improvement}
\label{app:efficiency_improvement}

\begin{figure*}[tb]
\centering
\includegraphics[width=0.46\columnwidth]{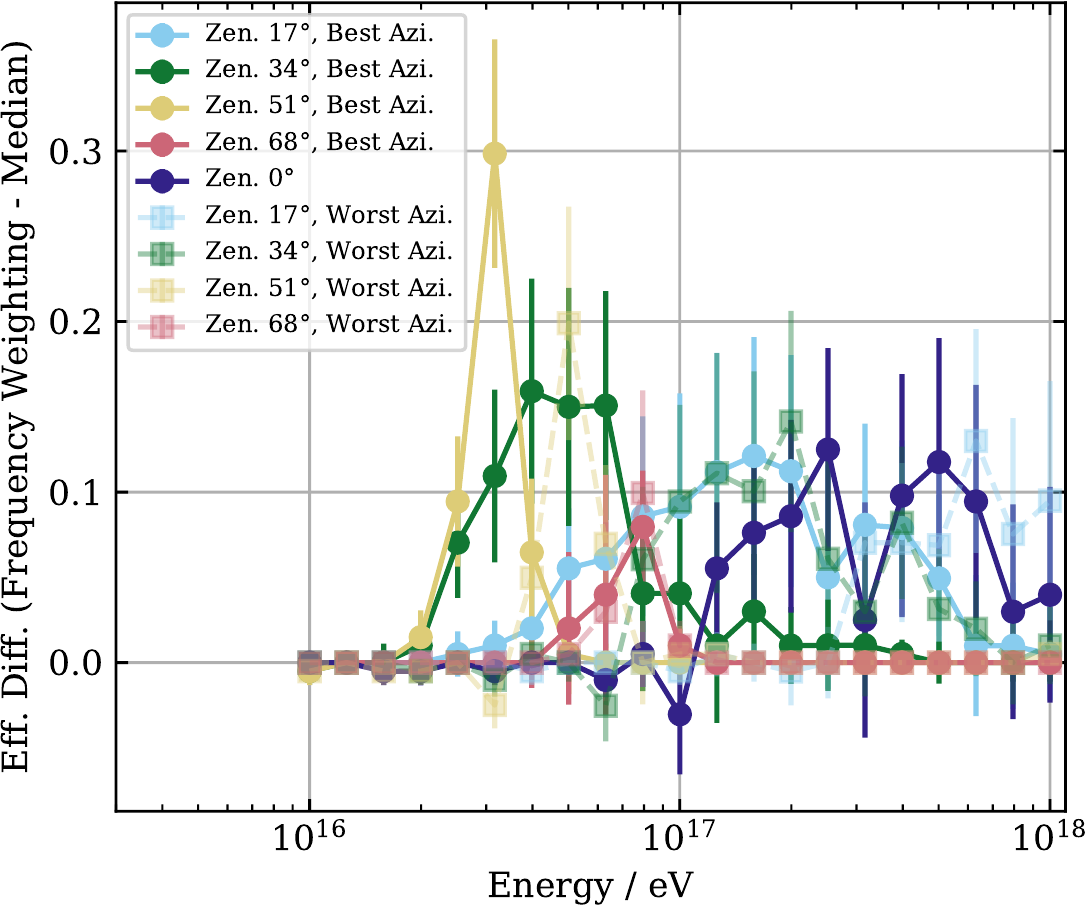}
\hspace{0.5cm}
\includegraphics[width=0.47\columnwidth]{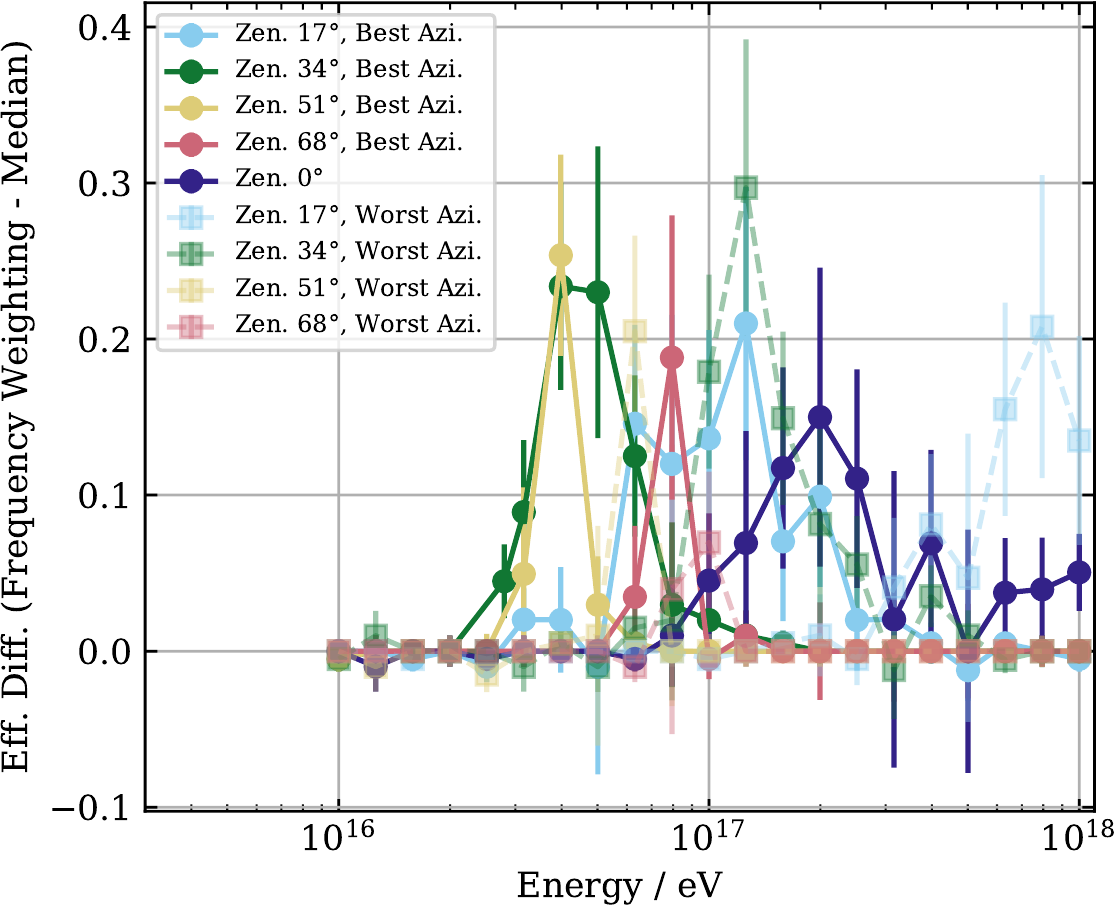}
\caption{The difference in reconstruction efficiency for proton (left) and iron (right) primaries are show, corresponding to the plots in \cref{fig:det_eff}.}
\label{fig:det_eff_diff}
\end{figure*}
As a method of verification of the frequency weighting scheme, the reconstruction efficiency of the IceTop Surface Enhancement was tested against the median filter method (\cref{eq:median_filter}).
The efficiency of the array was previously shown in \cref{fig:det_eff}.
In \cref{fig:det_eff} we show the difference in efficiency for the two methods.
The error bars are given by the Wilson confidence intervals.
The best- and worst-case azimuth angles correspond to the arrival directions where the geomagnetic angle is maximized and minimized, respectively.
A strict improvement in the detection efficiency of about 10 to 15\% is observed.
